# Supplementary material for: Signed Distance Field based Segmentation and Statistical Shape Modelling of the Left Atrial Appendage
Source: arXiv:2402.07708 source file (2024-02-12)
Supplement: Supplementary file 1 [file appendix.tex]

\section{LAA decoupling and automatic landmarks}\label{app:LM}
The method for LAA decoupling is a combination of global information by registering to a common template and local fine-tuning by choosing the plane with the lowest cross-sectional area when slivering the LAA neck. 
Figure \ref{fig:decoupling} shows 12 examples of the line that decouples the LAA from the LA. 
After decoupling the LAA, the edge-points that used to connect the LAA and LA are denoted the "decoupled edge". 

\begin{figure*}[htbp]
\centering
\includegraphics[width=\linewidth]{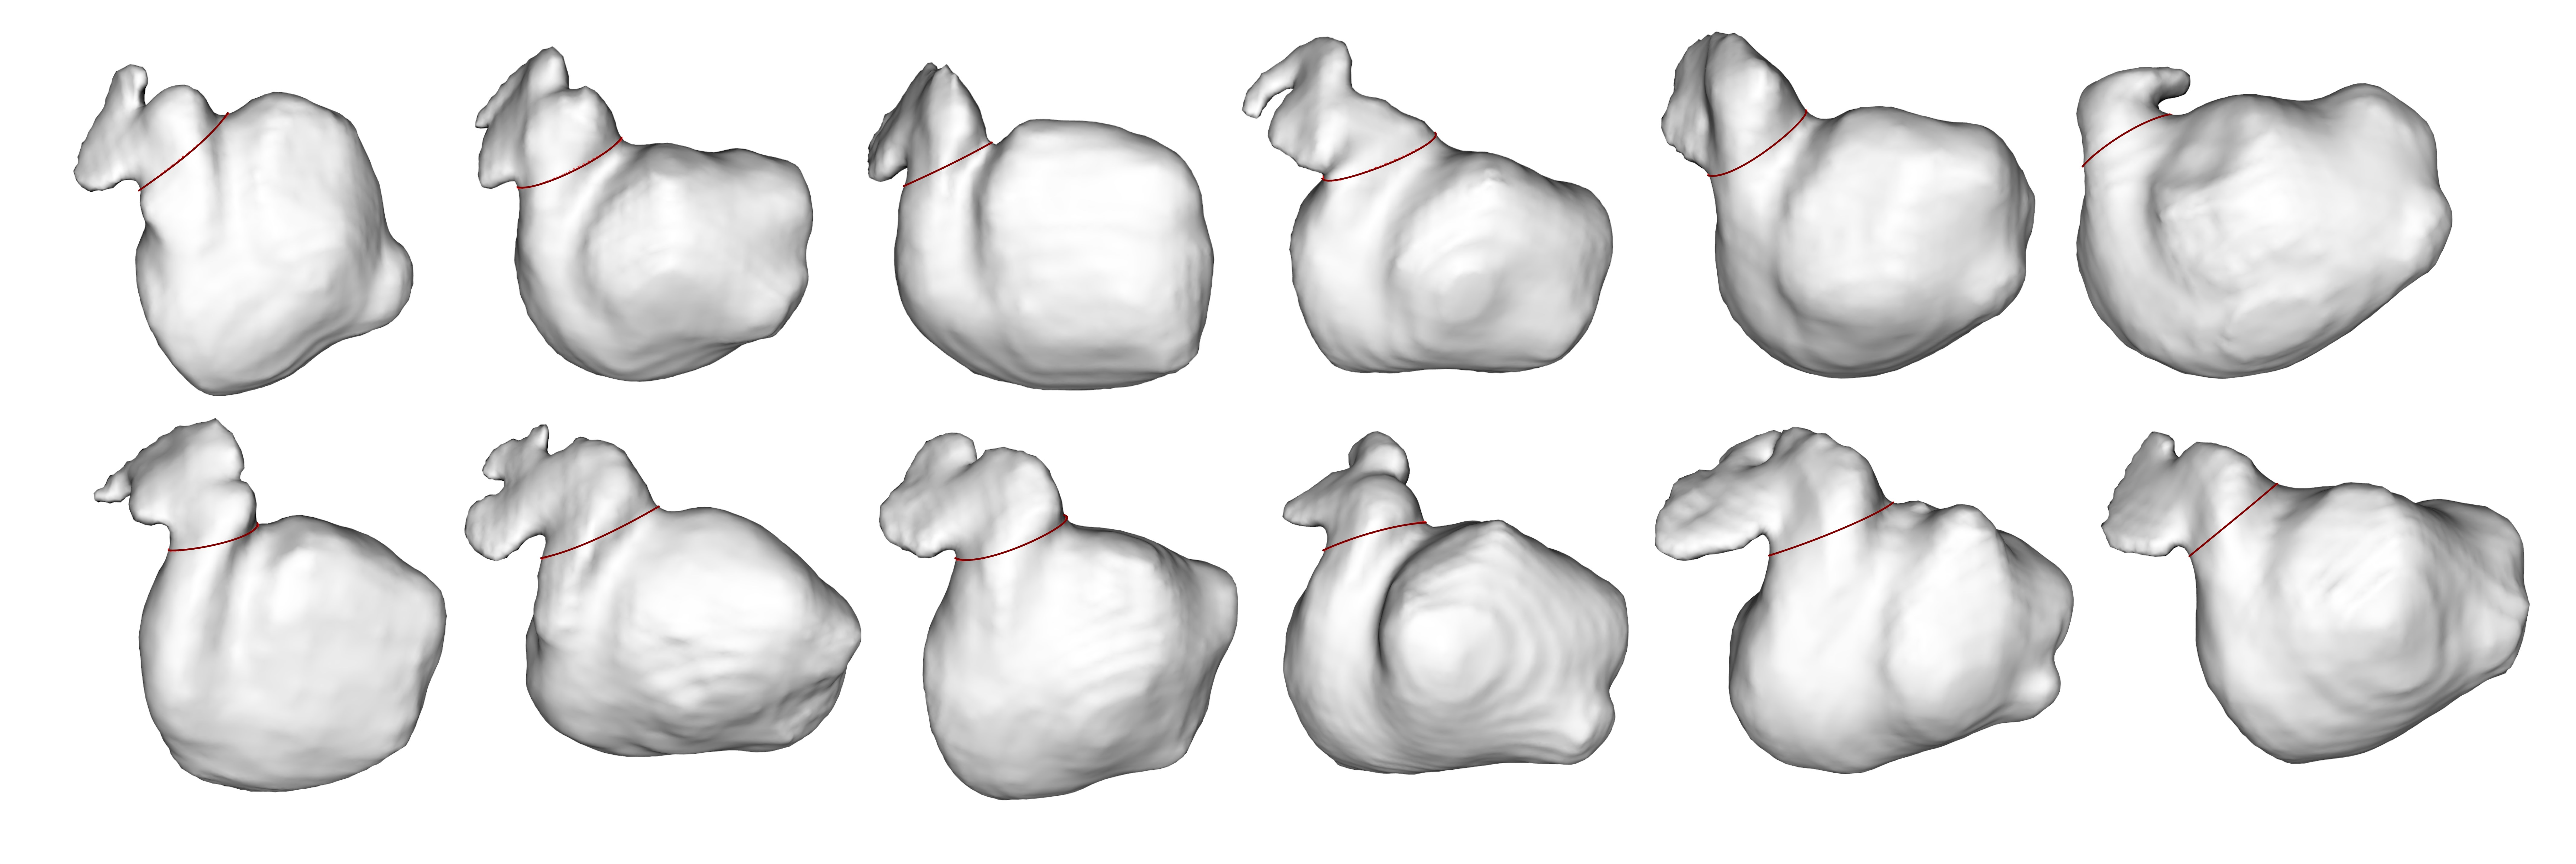}
\caption{12 randomly selected examples of lines separating the LAA from the LA.}
\label{fig:decoupling}
\end{figure*}

To aid the registration process we introduce five automatically derived landmarks on the decoupled LAA surface. 
%The first three landmarks are rigidly aligned with a landmark transform and the two remaining landmarks are assigned as number 4 and 5. 

\begin{figure}[htbp]
\centering
\includegraphics[width=0.5\linewidth]{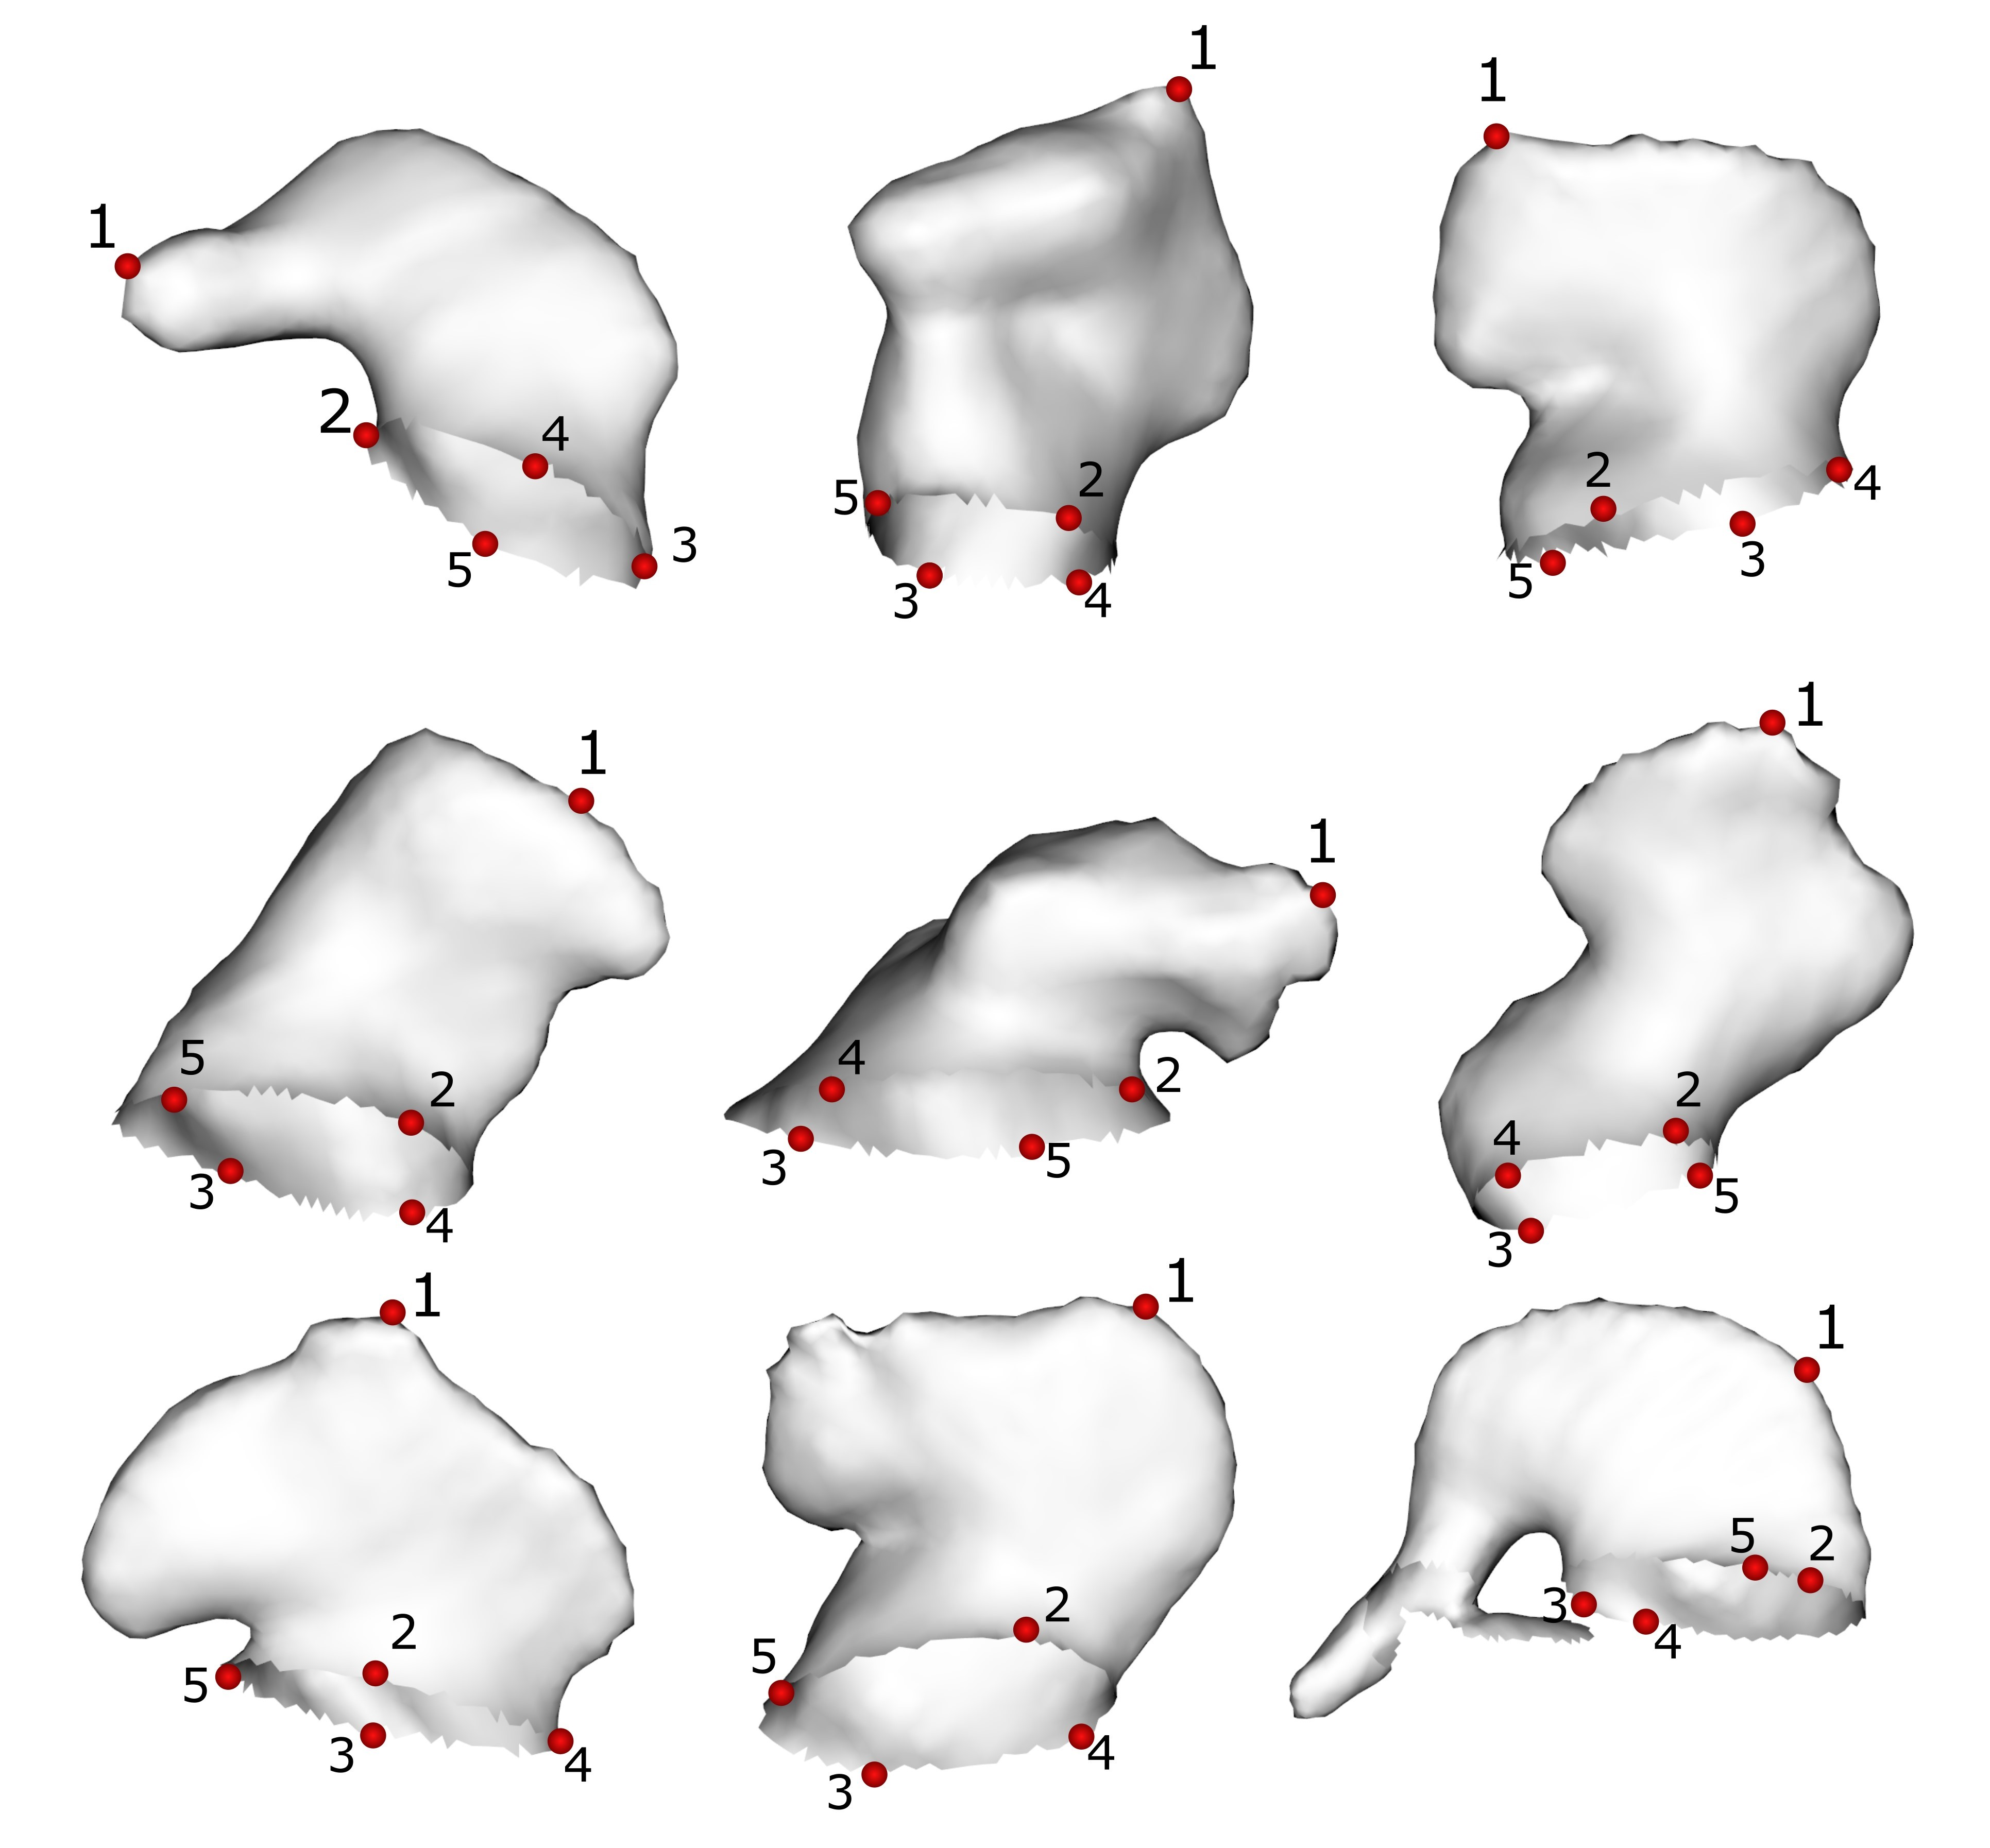}
\caption{Examples of landmarks placed with the automatic algorithm. The nine examples are the same as the LAAs in Figure \ref{fig:registration_results}, where they correspond to the best, median and worst results (row-wise) when registering to the common template.}
\label{fig:LM}
\end{figure}

Figure \ref{fig:LM} show nine examples of landmarks on LAA surfaces. 
The chosen examples correspond (row-wise) to the best, median and worst registration results.
